# Supplementary material for: Delphi: Efficient Asynchronous Approximate Agreement for Distributed Oracles
Source: arXiv:2405.02431 source file (2024-05-07)
Supplement: Supplementary file 1 [file avss-primitives.tex]

The adversarial strategy \adstrategy{1} will succeed if one honest node holds possession of \orderedsample{Y}{1}
%\textbf{Main intuitions}: To counter this power of the adversary, we propose a privacy-based approach to mitigate adversarial power. We use an Asynchronous Verifiable Secret Sharing (AVSS) scheme to reliably secret share input values of nodes. An AVSS scheme provides the following constructs that we utilize in our protocol.  Nodes run the first round of the protocol on information-private polynomial commitments of the values and reveal shares only after receiving $n-t$ witnesses on the information-private commitments. This forces the adversary to choose the message matrix without knowing honest nodes' values. 
We use Kate et al.'s \cite{kate2019brief} proposed AVSS scheme to generate constant-sized polynomial commitments for each of the secret generated by honest nodes. The AVSS scheme in \cite{kate2019brief} provides the following methods to generate a polynomial, a polynomial commitment, a secret share and a witness to testify that the share was evaluated on the polynomial. 
\begin{itemize}
    \item \textit{Setup}($1^{k}
    $,$n-t$) generates public parameters for all nodes. These parameters include a public algebraic structure and public private key pairs $<PK,SK>$ to commit to a polynomial of degree $n-t$. Let us denote these terms as System Parameters $SP$.
    \item \textit{PolyCommit(}$SP$,$\phi(x)$) outputs a constant sized commitment to the polynomial $\phi(x)$ using system parameters $SP$. The method generates commitment $C$ and associated decommitment information $aux$. 
    \item \textit{CreateWitness(}$SP$,$\phi(x)$,$i$,$aux$) outputs a pair of secret share and the witness to the polynomial $<i,\phi(i),w_i>$. An honest node generates $n$ share-witness pairs for every node participating in the protocol. 
    \item \textit{VerifyEval(}$SP,C,i,\phi(i),w_i$) verifies whether the share was generated using the polynomial $\phi(x)$ at point $i$. If so, the method outputs $accept$ else outputs $reject$. 
\end{itemize}
Consider an Asynchronous Verifiable Secret Sharing (AVSS) scheme with the following methods: 
\begin{enumerate}
    \item \textit{Setup($1^k,n-t$)} generates public parameters for all nodes for running an AVSS scheme. The method outputs setup parameters \textit{SP} that will be used to generate shares and commitments. The scheme is an $n-t$ threshold scheme which implies that at least $n-t$ nodes should reveal their shares to reveal a message. 
    \item \textit{Commit(SP,v)} generates a commitment to a value $v$ that should be secret shared. The method generates outputs $C$ which is the commitment to the value $v$. 
    \item \textit{CreateWitness(SP,v,i)} outputs a secret share for party $i$. \adithya{Party or node consistency.} The method outputs $s_i$ which is the secret share of the party $i$. \adithya{Party or node consistency.}
    \item \textit{VerifyShare(C,$s_i$)} verifies that the commitment $C$ and the secret share $s_i$ have been generated correctly. 
\end{enumerate}

% Extended protocol for RZ
\begin{enumerate}
    \item \textbf{Broadcast receive set.} Every node reliably broadcasts the set of first $n-f$ received and verified commitments. We name this variable $RC_i = R_i$. Every node reliably broadcasts received set message $RC_i$ to all other nodes. 
            \begin{gather}
                RC_i = R_i
            \end{gather}
            \begin{gather}
                RBroadcast(RC_i)
            \end{gather}
            \item \textbf{Wait for witnesses and reveal shares. } Before broadcasting a secret share of a reliably received commitment $j$, every honest node $i$ waits until all these conditions are satisfied:  
            \begin{enumerate}
                \item \textbf{Witnesses.} A node $j$ is a witness for node $i$ if the node $i$ has reliably received $RC_j$ AND $|RC_j \cap R_i| \ge n-f$. Every node waits until receiving $n-f$ witnesses. 
                \begin{gather}
                    Co_1 = |j| \ge n-f \ni \{|RC_j \cap R_i| \ge n-f\}
                \end{gather}
                \item A node $i$ waits until a commitment $C_j$ has been part of at least $n-f$ $RC_j$ messages. 
                \begin{gather}
                    Co_{2j} = |k| \ge n-f \ni \{C_j \in RC_k\} 
                \end{gather}
            \end{enumerate}
            Reveal share for commitment $C_j$ after both conditions $Co_1$ and $Co_{2j}$ are true. Broadcast share $s_{ij}$ after $Co_1 \cap Co_{2j}$
             \item \textbf{Wait for values to be revealed. } Every honest node $i$ waits to proceed to the next round, until the following conditions are true. 
            \begin{enumerate}
                \item Wait until reliably receiving commitments $C_j$ that have occurred in at least $t+1$ $RC$ messages. 
                \item Wait until all reliably received commitments are revealed. For a value to be revealed, $n-f$ nodes must broadcast their own secret shares. 
            \end{enumerate}
\end{enumerate}
