# Supplementary material for: Delphi: Efficient Asynchronous Approximate Agreement for Distributed Oracles
Source: arXiv:2405.02431 source file (2024-05-07)
Supplement: Supplementary file 2 [file messagematrix.tex]

\paragraph{Message Matrix}: The progress of the protocol can be represented as a matrix of messages reliably received by honest nodes at each step of the way. The following matrix $M$ is an example of the system's state before beginning the protocol. The system consists of $n = 7$ nodes with $f=2$ byzantine nodes and $h = 5$ honest nodes. The matrix denotes the  honest nodes' states and the messages they received from other honest nodes.  
$$ M = \begin{bmatrix}
1&0&0&0&0\\
0&1&0&0&0\\
0&0&1&0&0\\
0&0&0&1&0\\
0&0&0&0&1\\
\end{bmatrix}$$
An index $(i,j)$ in the matrix $M$ denotes whether the honest node $N_i$ received a message from another honest node $N_j$. Before the protocol begins, the state of the system is as described by $M$ because the nodes only have their messages. 

Witness technique protocol guarantees that after one round, there must be at least $f+1$ messages in common amongst all honest nodes. Representing this condition using the message matrix, there must be at least $f+1$ columns that must be completely $1$. In the above example, without the loss of generality, let the $f+1$ honest nodes be $1,2,3$. The message matrix will look like this:
$$M_1 = \begin{bmatrix}
1&1&1&0&0\\
1&1&1&0&0\\
1&1&1&0&0\\
1&1&1&1&0\\
1&1&1&0&1\\
\end{bmatrix}$$
$$M_1 = \begin{bmatrix}
1&1&0\\
1&1&0\\
1&1&1\\
\end{bmatrix}$$
The columns $1,2,3$ must be completely $1$. 
By the guarantees of witness technique, we can ensure that at least $n-2f$ columns must be fully $1$. However, the adversary can observe the values of honest nodes and decide which columns should be $1$. This property gives the adversary full power to decide where the value can converge in the range of honest nodes. As discussed in the introduction, certain ranges of values in the range of honest nodes might be more valuable (say closer to ground truth). Kate et al. ~\cite{kate2019brief} have discussed an Asynchronous Verifiable Secret Sharing (AVSS) scheme
