# Supplementary material for: Delphi: Efficient Asynchronous Approximate Agreement for Distributed Oracles
Source: arXiv:2405.02431 source file (2024-05-07)
Supplement: Supplementary file 3 [file rbroadcast.tex]

\subsection{Reliable Broadcast}
We discuss the reliable broadcast primitives in this subsection. We assume a set of nodes \noderange{1}{n} and a broadcasting node $i$ with an initial value $V$. The broadcaster node has access to a primitive \rbroadcast{i}{V} and every node $j$ participating in the protocol will deliver the $V$ by invoking \rdeliver{j}{V}. A protocol with these primitives is a reliable broadcast protocol if the following properties hold. 
\begin{itemize}
	\item \textit{Agreement}: If an honest node $i$ invokes \rdeliver{i}{V} and another honest node $j$ invokes \rdeliver{j}{V'}, then $V = V'$.
	\item \textit{Validity}: If the broadcasting node $i$ invokes \newline\rbroadcast{i}{V}, then every honest node $j$ eventually invokes \rdeliver{j}{V}. 
	\item \textit{Totality}: If an honest node $i$ invokes \rdeliver{i}{V}, then every other honest node $j$ will invoke \rdeliver{j}{V}.  
\end{itemize}
