# Supplementary material for: Delphi: Efficient Asynchronous Approximate Agreement for Distributed Oracles
Source: arXiv:2405.02431 source file (2024-05-07)
Supplement: Supplementary file 4 [file appendix.tex]

\appendix
